# Supplementary material for: BPO: Towards Balanced Preference Optimization between Knowledge Breadth and Depth in Alignment
Source: arXiv:2411.10914 source file (2025-02-20)
Supplement: Supplementary file 1 [file 4-method-appendix.tex]

In this section, we introduce our method Balanced Preference Optimization (\textsc{BPO}).

\textsc{BPO} balances knowledge by compressing knowledge breadth through selecting representative prompts via embedding-based clustering. 
Then, it generates responses and selects the informative ones to dynamically augment depth through gradient-based clustering.
Experiment results show that fine-tuning on refined knowledge leads to a better performance than the original data.
Our method entails two core steps:

\begin{itemize}
    \item \textit{knowledge breadth compression}: clustering the embedding vectors of prompts to select the most representative subset \( \mathcal{X_\text{rep}} \subset \mathcal{D}_{org} \) to compress the knowledge breadth. 
    \item \textit{dynamic knowledge depth augmentation}: we generate responses for the selected prompts to create a simplified solution space and use gradients to represent the uniformly increased samples. 
    Then, we evaluate the solution space by performing gradient clustering, which reflects the model's update directions, to dynamically allocate depth for different prompts.
\end{itemize}

\subsection{Knowledge Breadth Compression}
\label{prompts selection}

\paragraph{Embedding Vectors Computation} 
To reduce the breadth \( \mathcal{B} \) of the knowledge, we aim to select the most representative subset of prompts \( \mathcal{X_\text{rep}} \subset \mathcal{D}_\text{org} \). 
We achieve this by leveraging the embedding vectors of the prompts as representations.
Specifically, for each prompt \(x_i \in \mathcal{D}_\text{org} \), we obtain its embedding vector \(e_i\) using a pre-trained embedder \(f\) to represents sentences \citep{su2022one}, as follow:

\begin{equation} 
e_i = f(x_i) 
\end{equation}

% Thus, we have the embedding vector set \( \mathcal{E} = \{e_1, e_2, ..., e_n\} \).

\paragraph{Embedding Vectors Clustering} We then apply the \textit{K}-means clustering algorithm to the set of embedding vectors \( \{e_1, e_2, ..., e_n\} \) to partition them into 
\(C\) clusters \( \{ \mathcal{C}_1, \mathcal{C}_2, ..., \mathcal{C}_C \} \). 
Within each cluster \( \mathcal{C}_c \), we select the top \( \eta \) \% of prompts, based on Euclidean distance \( d(e_i, \mu_c) \), whose embedding vectors are closest to the centroid \(\mu_c\).
Formally, for each cluster \( \mathcal{C}_c \), we define the representative subset \( \mathcal{X}_c \) as:
\begin{equation} 
\small
\mathcal{X}_c = \left\{ x_i \in \mathcal{C}_c \ \bigg| \ \text{rank}\left( d(\mathbf{e}_i, \boldsymbol{\mu}_c) \right) \leq \eta \cdot |\mathcal{C}_c| \right\}
\label{rank}
\end{equation}
where \( |\mathcal{C}_c| \) is the number of data points in cluster \(\mathcal{C}_c\), and \(\text{rank}(\cdot)\) is the rank in ascending order of the distances. 
Then, we construct \({ \mathcal{X}_\textit{rep} = \bigcup_{c=1}^{C} \mathcal{X}_c}\).
This process effectively reduces the breadth \( \mathcal{B} \) to \( \mathcal{B}^{'} = |\mathcal{X}_\text{rep}| = \frac{\mathcal{B}}{s}\), focusing the knowledge on the most representative prompts, where \( s = \frac{1}{\eta} \) is the scaling ratio.
The results in Table \ref{tab: less prompt} demonstrate that only 5\% to 10\% prompts selected through embedding-based clustering can effectively align LLMs.

\subsection{Dynamic Knowledge Depth Augmentation}
\label{depth allocation}

\paragraph{Preliminary Supervised Fine-tuning with LoRA} 
This preliminary step involves fine-tuning the unsupervised base model \(\pi_0\) using a small, high-quality annotated seed dataset \( \mathcal{D}_{seed} = \{(x_1, y_1), \dots, (x_m, y_m)\} \), where \( x_i \) is the input text and \( y_i \) is the corresponding target output.
Additionally, we use LoRA~\citep{hu2021lora}, which reduces the number of trainable parameters by keeping the pre-trained model weights frozen and injecting trainable low-rank decomposition matrices into each layer.
This supervised fine-tuning (SFT) step effectively refines the base model, enhancing the subsequent DPO performance \citep{wang2024self,saeidi2024insights}. 
The fine-tuning objective is to minimize the supervised loss:

\begin{equation}
\small
\mathcal{L}_{\text{SFT}}(\theta) = \mathbb{E}_{(x_i, y_i) \sim \mathcal{D}_\text{seed}} \left[ - \log \pi_\theta(y_i \mid x_i) \right]
\label{sft}
\end{equation}

where \( \theta \) represents the model parameters.
After SFT, the fine-tuned policy is denoted as \( \pi_\theta = \pi_\text{SFT} \).

\paragraph{Uniform Depth Augmentation}
\label{pairs construction}
To increase the knowledge depth \( \mathcal{K} \), we construct additional response pairs for each prompt in the selected representative subset \(\mathcal{X}_{\text{rep}}\) from Section~\ref{prompts selection}. 
We generate multiple responses for each prompt \(x_i \in \mathcal{X}_{\text{rep}}\) using SFT policy \( \pi_\theta \) and employ GPT-4 to score these responses. 
By pairing responses with different scores, we construct all possible response pairs \((y_i^{p}, y_i^{q})\), where \(y_i^{p}\) and \(y_i^{q}\) have different scores. 
Considering that small score differences may not reflect meaningful distinctions due to potential inaccuracies in LLM judgments, it becomes difficult for the model to learn differences through DPO.
Consequently, we prioritize pairs with the largest score differences for each prompt \(x_i\).
Furthermore, since the base model has already been optimized for common scenarios, its responses are typically safe and exhibit minimal differences, making it challenging to generate response pairs with significant score differences. 
To address this for the safety dataset, we employed a different method by utilizing jailbreaking prompts to elicit more diverse responses. More details are provided in Section~\ref{comparision online generation}.
Thus, we uniformly expand the original knowledge depth \( \mathcal{K} = 2\) to \( \mathcal{K}^{'} = 2s \), achieving a uniform balance while maintaining the overall knowledge size, where \(s\) is the scaling ratio.
% Specifically, if we have reduced the breadth \(B\) to \(\frac{B}{M}\) by selecting only \(\frac{1}{M}\) of the prompts, we uniformly increase the depth $K$ by a factor of \(M\).
This process constructs a simplified solution space for \(\mathcal{X}_{\text{rep}}\), uniformly augmenting the depth \( \mathcal{K} \) of the knowledge.

\paragraph{Gradient Computation and Projection}
For the constructed solution space, we employ gradients to evaluate it. 
Building upon the previous uniform depth augmentation, we dynamically allocate the depth for each prompt \(x_i\) using the gradient features of each \textit{(prompt-response pair)}.
Following \citet{xia2024less}, we apply LoRA in the preliminary SFT step to reduce trainable parameters, and use random projection \citep{johnson1984extensions} to reduce the dimension of LoRA gradients.
Specifically, the parameter update based on the Adam optimizer \citep{kingma2014adam} is as follows:
\begin{equation}
\small
\theta^{t+1} - \theta^t = -\eta_t \Gamma(z, \theta^t)
\end{equation}
\begin{equation}
\small
\Gamma(z, \theta^t) \triangleq \frac{m^{t+1}}{\sqrt{v^{t+1}} + \epsilon}
\end{equation}
\begin{equation}
\small
m_{t+1} = \beta_1 m_t + (1 - \beta_1) \nabla \ell(z, \theta_t)
\end{equation}
\begin{equation}
\small
v_{t+1} = \beta_2 v_t + (1 - \beta_2) (\nabla \ell(z, \theta_t))^2
\end{equation}
\(\beta_1, \beta_2\) are the hyperparameters, \(\epsilon\) is a small constant, and \(\Gamma(z, \theta^t)\) represents the first-order expansion for the Adam dynamics.
Subsequently, for a given data sample \(z\) and model checkpoint \( \theta^t \), we use random projection \citep{johnson1984extensions} to map the high-dimensional LoRA gradients \(\nabla \ell(z; \theta^t)\) into a lower \textit{d}-dimensional space, denoted as \( \widehat{\nabla} \ell (z; \theta^t) \).
This enables a faster clustering step; the details are provided in Appendix \ref{app:random project}.
This gradient-based data representation allows us to measure the contribution of each response pair to the model's optimization, enabling a more efficient exploration of the solution space by dynamically adjusting the allocated the depth \(k_i\) for each prompt.

\begin{table*}[h]
\centering
\small
\begin{tabular}{ccccccccc}
\toprule[2pt]
\multirow{2}{*}{\textbf{Model}} & \multirow{2}{*}{\textbf{Method}} & \multicolumn{3}{c}{\textbf{safeRLHF}} & & \multicolumn{3}{c}{\textbf{HH-RLHF}} \\ \addlinespace[2pt] \cline{3-5}  \cline{7-9} \addlinespace[2pt]
 &  & \textbf{Data Size} & \textbf{MT-Bench}  & \textbf{AlpacaEval} & & \textbf{Data Size} & \textbf{MT-Bench}  & \textbf{AlpacaEval} \\ 
 \addlinespace[2pt] \hline  \addlinespace[2pt]
 
\multirow{7}{*}{$\text{Llama-3}_{\text{8B}}$}      
& Vanilla              & 50,489     & 4.90   & 36.84\%   &   & 27,000          & 4.71   & 18.14\%     \\ 
& KBC (\(s\)=10\%)     & 5,094     & 5.12   & 45.75\%    &   & 2744          & 4.11   & 20.12\%     \\ 
& Uniform Balance      & 45,522     & 5.19   & 46.18\%   &   & 32,928          & 4.42   & 25.34\%     \\ 
& random10\% UB        & 4,552     & 5.02   & 43.48\%    &   & 3,292          & 4.21   & 23.75\%     \\ 
& Curry-DPO            & 45,522    & 5.21   & 44.03\%    &   & 32,928   & 4.67   & 28.29\%     \\
& RS-DPO               & 5,2067    & 5.32   & 47.48\%    &   & 34,177       & 5.12   & 33.31\%     \\ 
& \textsc{BPO} (Ours)  & 4,570      & \textbf{5.45}   & \textbf{48.24\% } &  & 3,312     & \textbf{5.48 }  & \textbf{40.25\%}
\\ \addlinespace[2pt] \hdashline[1pt/1pt] \addlinespace[2pt]

\multirow{7}{*}{$\text{Llama-2}_{\text{13B}}$} 
& Vanilla              & 50,489     & 5.40   & 48.07\%  &  & 27,000        & 5.79   & 21.50\%     \\ 
& KBC (\(s\)=10\%)     & 5,094      & 5.38   & 46.71\%  &  & 2744          & 5.14   & 22.85\%     \\ 
& Uniform Balance      & 29,555     & 5.68   & 50.30\%  &  & 26,792        & 5.51   & 24.68\%     \\ 
& random10\% UB        & 2,955      & 4.02   & 48.64\%  &  & 2,679         & 4.64   & 21.11\%     \\ 
& Curry-DPO            & 2,9555     & 5.67   & 48.50\%  &  & 26,792        & 5.59   & 24.22\%     \\
& RS-DPO               & 49,664     & 5.79   & 50.73\%  &  & 27,143        & \textbf{5.83}   & 25.26\%     \\ 
& \textsc{BPO} (Ours)  & 3,042     & \textbf{5.85}   & \textbf{54.27\%}  & & 2,753          & 5.74   & \textbf{26.96\%}
\\ \bottomrule[2pt]
\end{tabular}
\caption{Performance comparison of different pair selection strategies on the SafeRLHF and HH-RLHF datasets.
% The performance is evaluated on MT-Bench with the average scores of round 1 and round 2, and the win rate on AlpacaEval against text-davinci-003.
}
\label{tab: main exp}
\end{table*}

\paragraph{Dynamic Depth Allocation}
We perform \textit{K}-means clustering on the set of gradient features \( \widehat{\nabla} \ell (z; \theta_t) \) into \( G \) clusters \( \{ G_1, G_2, \ldots, G_G \} \) to evaluate the solution space from the perspective of model updates. 
For each cluster \( G_g \), we select the top \( \eta \% \) of \textit{(prompt, response pair)} whose gradient vectors are closest to the cluster centroid \( \boldsymbol{\mu}_g \), based on the Euclidean distance. 
The selected subset \( S_g \) for cluster \( G_g \) is the same as Equation \ref{rank}, and we construct \({\scriptstyle \mathcal{D}_{dyn} = \bigcup_{g=1}^{G} \mathcal{S}_g}\).
This selection process ensures that \( \mathcal{D}_{dyn} \) is informative of the diverse update directions in the solution space and effectively reduces the training samples to a smaller size.

\begin{figure}[h]
    \centering
    \scalebox{0.25}{\includegraphics{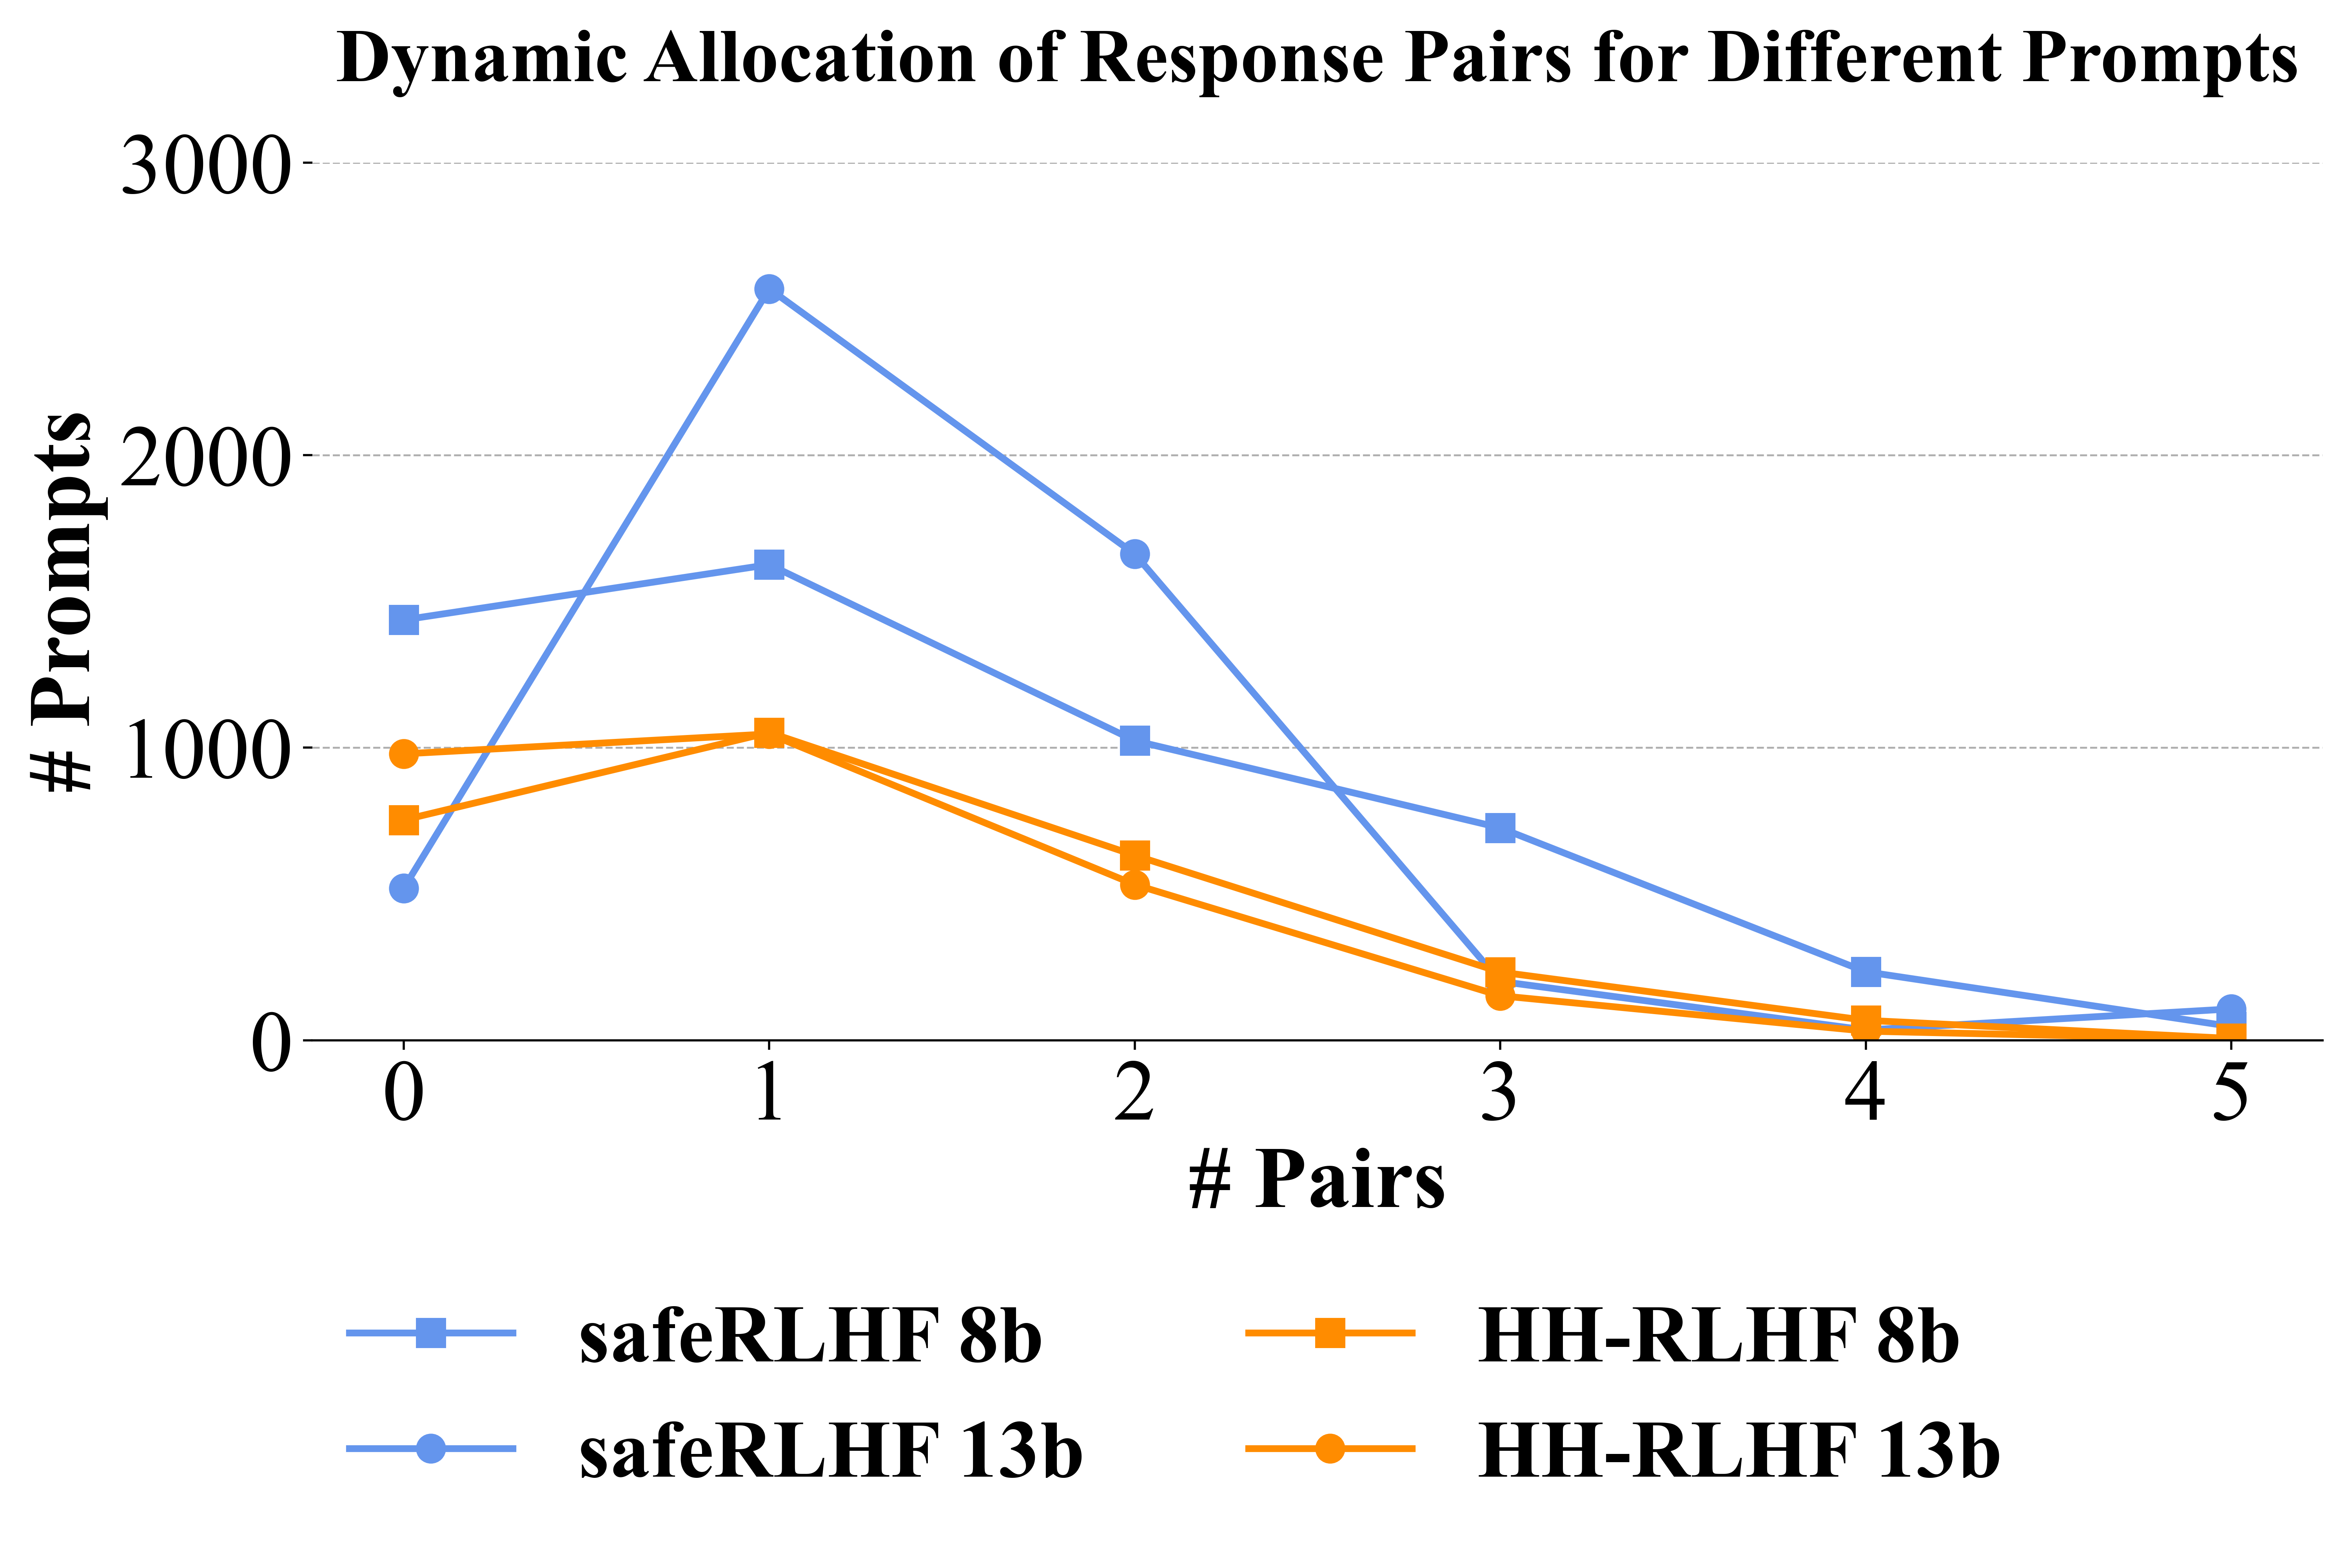} }
    \caption{
Dynamic allocation of response pairs based on gradient clustering. The result illustrates how \textsc{BPO} optimizes the knowledge depth for different prompts.
    }
    \label{fig:dynamic}
\end{figure}

The final set of informative response pairs refines the knowledge, allowing the model to learn more efficiently and achieve better alignment during fine-tuning.
Figure~\ref{fig:dynamic} shows the dynamic allocation of response pairs for different prompts, where the number of pairs varies based on the clustering results and gradient-based selection. 
This illustrates how the model dynamically adjusts the number of response pairs for different prompts to optimize the knowledge depth.
We then perform DPO fine-tuning using these selected response pairs, which leads to better alignment and performance improvements as demonstrated in our experiments.
